# Supplementary material for: High-resolution Face Swapping via Latent Semantics Disentanglement
Source: arXiv:2203.15958 source file (2022-03-30)
Supplement: Supplementary file 1 [file supp_video.tex]

\begin{figure*}[t]
   \centering
     \captionsetup[subfigure]{labelformat=empty,justification=centering}
     \vspace{-7mm}
     \begin{subfigure}{.16\linewidth}
     \centering
     \vspace{10mm}
     \includegraphics[width=\linewidth]{supp/videos/sample1/source}\vspace{-1mm}\caption{source}
     \includegraphics[width=\linewidth]{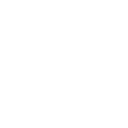}
     \includegraphics[width=\linewidth]{figure/video/white}
     \end{subfigure}
     \begin{subfigure}{.16\linewidth}
     \centering
     \includegraphics[width=\linewidth]{supp/videos/sample1/source/000000}
     \includegraphics[width=\linewidth]{supp/videos/sample1/megafs/frame0000}
     \includegraphics[width=\linewidth]{supp/videos/sample1/ours/frame0000}
     \end{subfigure}
     \hspace{-2mm}
     \begin{subfigure}{.16\linewidth}
     \centering
     \includegraphics[width=\linewidth]{supp/videos/sample1/source/000055}
     \includegraphics[width=\linewidth]{supp/videos/sample1/megafs/frame0055}
     \includegraphics[width=\linewidth]{supp/videos/sample1/ours/frame0055}
     \end{subfigure}
     \hspace{-2mm}
     \begin{subfigure}{.16\linewidth}
     \centering
     \includegraphics[width=\linewidth]{supp/videos/sample1/source/000102}
     \includegraphics[width=\linewidth]{supp/videos/sample1/megafs/frame0102}
     \includegraphics[width=\linewidth]{supp/videos/sample1/ours/frame0102}
     \end{subfigure}
     \hspace{-2mm}
     \begin{subfigure}{.16\linewidth}
     \centering
     \includegraphics[width=\linewidth]{supp/videos/sample1/source/000008}
     \includegraphics[width=\linewidth]{supp/videos/sample1/megafs/frame0008}
     \includegraphics[width=\linewidth]{supp/videos/sample1/ours/frame0008}
     \end{subfigure}
     \hspace{-2mm}
     \begin{subfigure}{.16\linewidth}
     \centering
     \includegraphics[width=\linewidth]{supp/videos/sample1/source/000108}
     \includegraphics[width=\linewidth]{supp/videos/sample1/megafs/frame0108}
     \includegraphics[width=\linewidth]{supp/videos/sample1/ours/frame0109}
     \end{subfigure}
     \rotatebox[origin=c]{270}{{Target} \hspace{15mm} MegaFS \hspace{15mm} Ours}
     \vspace{-5mm}
     \caption{Qualitative comparison of video face swapping with MegaFS.}
     \label{fig.video_img}
\end{figure*}
